# Supplementary material for: Theory of voltammetry in charged porous media
Source: arXiv:1709.05073 ancillary file (2018-01-21)
Supplement: Supplementary file 1 [file supplementary.pdf]

# Theory of voltammetry in charged porous media: supplementary material

Edwin Khoo[1] and Martin Z. Bazant[1,2,*]

[1] *Department of Chemical Engineering, Massachusetts Institute of Technology, Cambridge, MA 02139, USA*

[2] *Department of Mathematics, Massachusetts Institute of Technology, Cambridge, MA 02139, USA*

(Dated: January 19, 2018)

* Corresponding author: bazant@mit.edu

## I. CONSTRUCTION OF STEADY STATE EQUATIONS FOR USE IN MATLAB

Throughout this section, we use dimensionless variables. To avoid cluttering the notation, we drop tildes on all dimensionless variables and the $-$ subscript on $\tilde{c}_-$. MATLAB's `bvp4c` function solves boundary value problems of the form

$$\frac{\mathrm{d}y}{\mathrm{d}x} = f(x, y, p), \quad y_{\mathrm{BC}} = 0, \tag{1}$$

where $x$ is the scalar independent variable, $y$ is the vector of dependent variables, $p$ is the vector of parameters, $f$ is the vector function relating $\frac{\mathrm{d}y}{\mathrm{d}x}$ to $x$, $y$ and $p$, and $y_{\mathrm{BC}}$ is the vector of boundary conditions. Different boundary conditions result in different expressions for $y$, $p$, $f$ and $y_{\mathrm{BC}}$. Throughout this section, we use primes to denote derivatives taken with respect to $x$. We first provide the expression for $J$, which will be used throughout the section:

$$J = \beta_{\mathrm{D}}[(D_{-0} - D_{+0})c' - (z_+ D_{+0} - z_- D_{-0})c\phi' + z_+ D_{+0}\rho_{\mathrm{s}}\phi'], \tag{2}$$

$$\beta_{\mathrm{D}} = -\frac{z_- D_{-0}}{2(z_+ D_{+0} - z_- D_{-0})}. \tag{3}$$

### A. Case 1: reservoir boundary condition at anode

$p$ is not required and $y$ and $f$ are given by:

$$y = \begin{bmatrix} c \\ c' \\ \phi \\ \phi' \end{bmatrix}, \tag{4}$$

$$f = \begin{bmatrix} c' \\ c'' \\ \phi' \\ \phi'' \end{bmatrix} = \begin{bmatrix} c' \\ \frac{z_+ z_- \rho_{\mathrm{s}} c' \phi'}{(z_+ - z_-)c - z_+ \rho_{\mathrm{s}}} \\ \phi' \\ -\frac{(z_+ - z_-)c'\phi'}{(z_+ - z_-)c - z_+ \rho_{\mathrm{s}}} \end{bmatrix}. \tag{5}$$

For galvanostatic conditions where we impose $J(x = 1) = I_{\mathrm{applied}}$,

$$y_{\mathrm{BC}} = \begin{bmatrix} c(x = 0) - \beta_1 \\ \phi(x = 0) \\ c' + z_- c\phi'|_{x=1} \\ I_{\mathrm{applied}} - J(x = 1) \end{bmatrix}, \tag{6}$$

while for potentiostatic conditions where we impose $\phi(x=1)=-V$,

$$y_{\mathrm{BC}} = \begin{bmatrix} c(x=0)-\beta_1 \\ \phi(x=0) \\ c' + z_- c\phi'|_{x=1} \\ \phi(x=1)+V \end{bmatrix}. \tag{7}$$

### B. Case 2: no-anion-flux boundary condition at anode

We need to add a new variable to $y$ that enforces the integral constraint for the conservation of the number of anions. This variable is simply called $y_5$ as it is the 5th element of $y$. $p$ is not required and $y$ and $f$ are given by:

$$y = \begin{bmatrix} c \\ c' \\ \phi \\ \phi' \\ y_5 \end{bmatrix}, \tag{8}$$

$$f = \begin{bmatrix} c' \\ c'' \\ \phi' \\ \phi'' \\ c \end{bmatrix} = \begin{bmatrix} c' \\ \frac{z_+ z_- \rho_{\mathrm{s}} c' \phi'}{(z_+ - z_-)c - z_+ \rho_{\mathrm{s}}} \\ \phi' \\ -\frac{(z_+ - z_-)c'\phi'}{(z_+ - z_-)c - z_+ \rho_{\mathrm{s}}} \\ c \end{bmatrix}. \tag{9}$$

For galvanostatic conditions where we impose $J(x=1)=I_{\mathrm{applied}}$,

$$y_{\mathrm{BC}} = \begin{bmatrix} y_5(x=0) \\ \phi(x=0) \\ c' + z_- c\phi'|_{x=1} \\ I_{\mathrm{applied}} - J(x=1) \\ y_5(x=1)-\beta_1 \end{bmatrix}, \tag{10}$$

while for potentiostatic conditions where we impose $\phi(x=1)=-V$,

$$y_{\mathrm{BC}}=\begin{bmatrix} y_5(x=0) \\ \phi(x=0) \\ c'+z_-c\phi'\big|_{x=1} \\ \phi(x=1)+V \\ y_5(x=1)-\beta_1 \end{bmatrix}. \tag{11}$$

### C. Case 3: Butler-Volmer boundary conditions at anode and cathode

Like in case 2, we need to add a new variable to $y$, which is called $y_5$, that enforces the integral constraint for the conservation of the number of anions. $p$ is needed for galvanostatic conditions where we impose $J(x=1)=I_{\mathrm{applied}}$ in order to find $V$ (recall that $\phi_{\mathrm{e}}^{\mathrm{c}}=-V$) while $p$ is not required for potentiostatic conditions where we impose $\phi_{\mathrm{e}}^{\mathrm{c}}=-V$. $y$ and $f$ are given by:

$$y=\begin{bmatrix} c \\ c' \\ \phi \\ \phi' \\ y_5 \end{bmatrix}, \tag{12}$$

$$f=\begin{bmatrix} c' \\ c'' \\ \phi' \\ \phi'' \\ c \end{bmatrix}=\begin{bmatrix} c' \\ \frac{z_+z_-\rho_{\mathrm{s}}c'\phi'}{(z_+-z_-)c-z_+\rho_{\mathrm{s}}} \\ \phi' \\ -\frac{(z_+-z_-)c'\phi'}{(z_+-z_-)c-z_+\rho_{\mathrm{s}}} \\ c \end{bmatrix}. \tag{13}$$

For galvanostatic conditions where we impose $J(x=1)=I_{\text{applied}}$,

$$p = V, \tag{14}$$

$$y_{\text{BC}} = \begin{bmatrix} y_5(x=0) \\ J(x=0)+J_{\text{F}}^{\text{a}} \\ c' + z_- c\phi'|_{x=1} \\ -J(x=1)+J_{\text{F}}^{\text{c}} \\ y_5(x=1)-\beta_1 \\ I_{\text{applied}} - J(x=1) \end{bmatrix}, \tag{15}$$

while for potentiostatic conditions where we impose $\phi_{\text{e}}^{\text{c}} = -V$,

$$y_{\text{BC}} = \begin{bmatrix} y_5(x=0) \\ J(x=0)+J_{\text{F}}^{\text{a}} \\ c' + z_- c\phi'|_{x=1} \\ -J(x=1)+J_{\text{F}}^{\text{c}} \\ y_5(x=1)-\beta_1 \end{bmatrix}. \tag{16}$$

## II. JACOBIANS FOR STEADY STATE EQUATIONS

To increase convergence speed, we provide Jacobians to the `bvp4c` function. There are two types of Jacobians we can provide: 1) partial derivatives of $f$ with respect to $y$ and $p$ ($\frac{\partial f}{\partial y}$ and $\frac{\partial f}{\partial p}$), and 2) partial derivatives of $y_{\text{BC}}$ with respect to $y(x=0)$, $y(x=1)$ and $p$ ($\frac{\partial y_{\text{BC}}}{\partial y(x=0)}$, $\frac{\partial y_{\text{BC}}}{\partial y(x=1)}$ and $\frac{\partial y_{\text{BC}}}{\partial p}$). For simplicity, the elements of $f$, $y$, $y_{\text{BC}}$, $y(x=0)$ and $y(x=1)$

are written as:

$$f = \begin{bmatrix} f_1 \\ f_2 \\ f_3 \\ f_4 \end{bmatrix} \quad \text{or} \quad \begin{bmatrix} f_1 \\ f_2 \\ f_3 \\ f_4 \\ f_5 \end{bmatrix}, \tag{17}$$

$$y = \begin{bmatrix} y_1 \\ y_2 \\ y_3 \\ y_4 \end{bmatrix} \quad \text{or} \quad \begin{bmatrix} y_1 \\ y_2 \\ y_3 \\ y_4 \\ y_5 \end{bmatrix}, \tag{18}$$

$$y_{\mathrm{BC}} = \begin{bmatrix} y_{\mathrm{BC},1} \\ y_{\mathrm{BC},2} \\ y_{\mathrm{BC},3} \\ y_{\mathrm{BC},4} \end{bmatrix} \quad \text{or} \quad \begin{bmatrix} y_{\mathrm{BC},1} \\ y_{\mathrm{BC},2} \\ y_{\mathrm{BC},3} \\ y_{\mathrm{BC},4} \\ y_{\mathrm{BC},5} \end{bmatrix} \quad \text{or} \quad \begin{bmatrix} y_{\mathrm{BC},1} \\ y_{\mathrm{BC},2} \\ y_{\mathrm{BC},3} \\ y_{\mathrm{BC},4} \\ y_{\mathrm{BC},5} \\ y_{\mathrm{BC},6} \end{bmatrix}, \tag{19}$$

$$y(x=0) = \begin{bmatrix} y_{0,1} \\ y_{0,2} \\ y_{0,3} \\ y_{0,4} \end{bmatrix} \quad \text{or} \quad \begin{bmatrix} y_{0,1} \\ y_{0,2} \\ y_{0,3} \\ y_{0,4} \\ y_{0,5} \end{bmatrix}, \tag{20}$$

$$y(x=1) = \begin{bmatrix} y_{1,1} \\ y_{1,2} \\ y_{1,3} \\ y_{1,4} \end{bmatrix} \quad \text{or} \quad \begin{bmatrix} y_{1,1} \\ y_{1,2} \\ y_{1,3} \\ y_{1,4} \\ y_{1,5} \end{bmatrix}. \tag{21}$$

### A. Case 1: reservoir boundary condition at anode

The nonzero elements of the $\frac{\partial f}{\partial y}$ Jacobian $\in \mathbb{R}^{4\times4}$ are given by:

$$\frac{\partial f_1}{\partial y_2} = 1, \tag{22}$$

$$\frac{\partial f_2}{\partial y_1} = -\frac{(z_+ - z_-)z_+z_-\rho_\mathrm{s}c'\phi'}{[(z_+ - z_-)c - z_+\rho_\mathrm{s}]^2}, \tag{23}$$

$$\frac{\partial f_2}{\partial y_2} = \frac{z_+z_-\rho_\mathrm{s}\phi'}{(z_+ - z_-)c - z_+\rho_\mathrm{s}}, \tag{24}$$

$$\frac{\partial f_2}{\partial y_4} = \frac{z_+z_-\rho_\mathrm{s}c'}{(z_+ - z_-)c - z_+\rho_\mathrm{s}}, \tag{25}$$

$$\frac{\partial f_3}{\partial y_4} = 1, \tag{26}$$

$$\frac{\partial f_4}{\partial y_1} = \frac{(z_+ - z_-)^2c'\phi'}{[(z_+ - z_-)c - z_+\rho_\mathrm{s}]^2}, \tag{27}$$

$$\frac{\partial f_4}{\partial y_2} = -\frac{(z_+ - z_-)\phi'}{(z_+ - z_-)c - z_+\rho_\mathrm{s}}, \tag{28}$$

$$\frac{\partial f_4}{\partial y_4} = -\frac{(z_+ - z_-)c'}{(z_+ - z_-)c - z_+\rho_\mathrm{s}}. \tag{29}$$

The nonzero elements of the $\frac{\partial y_\mathrm{BC}}{\partial y(x=0)}$ Jacobian $\in \mathbb{R}^{4\times4}$ are given by:

$$\frac{\partial y_\mathrm{BC,1}}{\partial y_{0,1}} = 1, \tag{30}$$

$$\frac{\partial y_\mathrm{BC,2}}{\partial y_{0,3}} = 1. \tag{31}$$

For galvanostatic conditions, the nonzero elements of the $\frac{\partial y_\mathrm{BC}}{\partial y(x=1)}$ Jacobian $\in \mathbb{R}^{4\times4}$ are given by

$$\frac{\partial y_\mathrm{BC,3}}{\partial y_{1,1}} = z_-\phi'(x=1), \tag{32}$$

$$\frac{\partial y_\mathrm{BC,3}}{\partial y_{1,2}} = 1, \tag{33}$$

$$\frac{\partial y_\mathrm{BC,3}}{\partial y_{1,4}} = z_-c(x=1), \tag{34}$$

$$\frac{\partial y_\mathrm{BC,4}}{\partial y_{1,1}} = \beta_\mathrm{D}(z_+D_{+0} - z_-D_{-0})\phi'(x=1), \tag{35}$$

$$\frac{\partial y_\mathrm{BC,4}}{\partial y_{1,2}} = -\beta_\mathrm{D}(D_{-0} - D_{+0}), \tag{36}$$

$$\frac{\partial y_\mathrm{BC,4}}{\partial y_{1,4}} = -\beta_\mathrm{D}[-(z_+D_{+0} - z_-D_{-0})c(x=1) + z_+D_{+0}\rho_\mathrm{s}], \tag{37}$$

while for potentiostatic conditions, the nonzero elements of the $\frac{\partial y_{\mathrm{BC}}}{\partial y(x=1)}$ Jacobian $\in \mathbb{R}^{4\times 4}$ are given by

$$\frac{\partial y_{\mathrm{BC},3}}{\partial y_{1,1}} = z_- \phi'(x=1), \tag{38}$$

$$\frac{\partial y_{\mathrm{BC},3}}{\partial y_{1,2}} = 1, \tag{39}$$

$$\frac{\partial y_{\mathrm{BC},3}}{\partial y_{1,4}} = z_- c(x=1), \tag{40}$$

$$\frac{\partial y_{\mathrm{BC},4}}{\partial y_{1,3}} = 1. \tag{41}$$

### B. Case 2: no-anion-flux boundary condition at anode

The nonzero elements of the $\frac{\partial f}{\partial y}$ Jacobian $\in \mathbb{R}^{5\times 5}$ are given by:

$$\frac{\partial f_1}{\partial y_2} = 1, \tag{42}$$

$$\frac{\partial f_2}{\partial y_1} = -\frac{(z_+ - z_-) z_+ z_- \rho_{\mathrm{s}} c' \phi'}{\left[(z_+ - z_-)c - z_+ \rho_{\mathrm{s}}\right]^2}, \tag{43}$$

$$\frac{\partial f_2}{\partial y_2} = \frac{z_+ z_- \rho_{\mathrm{s}} \phi'}{(z_+ - z_-)c - z_+ \rho_{\mathrm{s}}}, \tag{44}$$

$$\frac{\partial f_2}{\partial y_4} = \frac{z_+ z_- \rho_{\mathrm{s}} c'}{(z_+ - z_-)c - z_+ \rho_{\mathrm{s}}}, \tag{45}$$

$$\frac{\partial f_3}{\partial y_4} = 1, \tag{46}$$

$$\frac{\partial f_4}{\partial y_1} = \frac{(z_+ - z_-)^2 c' \phi'}{\left[(z_+ - z_-)c - z_+ \rho_{\mathrm{s}}\right]^2}, \tag{47}$$

$$\frac{\partial f_4}{\partial y_2} = -\frac{(z_+ - z_-)\phi'}{(z_+ - z_-)c - z_+ \rho_{\mathrm{s}}}, \tag{48}$$

$$\frac{\partial f_4}{\partial y_4} = -\frac{(z_+ - z_-)c'}{(z_+ - z_-)c - z_+ \rho_{\mathrm{s}}}, \tag{49}$$

$$\frac{\partial f_5}{\partial y_1} = 1. \tag{50}$$

The nonzero elements of the $\frac{\partial y_{\mathrm{BC}}}{\partial y(x=0)}$ Jacobian $\in \mathbb{R}^{5\times 5}$ are given by:

$$\frac{\partial y_{\mathrm{BC},1}}{\partial y_{0,5}} = 1, \tag{51}$$

$$\frac{\partial y_{\mathrm{BC},2}}{\partial y_{0,3}} = 1. \tag{52}$$

For galvanostatic conditions, the nonzero elements of the $\frac{\partial y_{\mathrm{BC}}}{\partial y(x=1)}$ Jacobian $\in \mathbb{R}^{5\times 5}$ are given by

$$\frac{\partial y_{\mathrm{BC},3}}{\partial y_{1,1}} = z_- \phi'(x=1), \tag{53}$$
$$\frac{\partial y_{\mathrm{BC},3}}{\partial y_{1,2}} = 1, \tag{54}$$
$$\frac{\partial y_{\mathrm{BC},3}}{\partial y_{1,4}} = z_- c(x=1), \tag{55}$$
$$\frac{\partial y_{\mathrm{BC},4}}{\partial y_{1,1}} = \beta_{\mathrm{D}}(z_+ D_{+0} - z_- D_{-0})\phi'(x=1), \tag{56}$$
$$\frac{\partial y_{\mathrm{BC},4}}{\partial y_{1,2}} = -\beta_{\mathrm{D}}(D_{-0} - D_{+0}), \tag{57}$$
$$\frac{\partial y_{\mathrm{BC},4}}{\partial y_{1,4}} = -\beta_{\mathrm{D}}[-(z_+ D_{+0} - z_- D_{-0})c(x=1) + z_+ D_{+0}\rho_{\mathrm{s}}], \tag{58}$$
$$\frac{\partial y_{\mathrm{BC},5}}{\partial y_{1,5}} = 1, \tag{59}$$

while for potentiostatic conditions, the nonzero elements of the $\frac{\partial y_{\mathrm{BC}}}{\partial y(x=1)}$ Jacobian $\in \mathbb{R}^{5\times 5}$ are given by

$$\frac{\partial y_{\mathrm{BC},3}}{\partial y_{1,1}} = z_- \phi'(x=1), \tag{60}$$
$$\frac{\partial y_{\mathrm{BC},3}}{\partial y_{1,2}} = 1, \tag{61}$$
$$\frac{\partial y_{\mathrm{BC},3}}{\partial y_{1,4}} = z_- c(x=1), \tag{62}$$
$$\frac{\partial y_{\mathrm{BC},4}}{\partial y_{1,3}} = 1, \tag{63}$$
$$\frac{\partial y_{\mathrm{BC},5}}{\partial y_{1,5}} = 1. \tag{64}$$

### C. Case 3: Butler-Volmer boundary conditions at anode and cathode

The nonzero elements of the $\frac{\partial f}{\partial y}$ Jacobian $\in \mathbb{R}^{5\times 5}$ are given by:

$$\frac{\partial f_1}{\partial y_2} = 1, \tag{65}$$

$$\frac{\partial f_2}{\partial y_1} = -\frac{(z_+ - z_-)z_+ z_- \rho_\mathrm{s} c' \phi'}{[(z_+ - z_-)c - z_+\rho_\mathrm{s}]^2}, \tag{66}$$

$$\frac{\partial f_2}{\partial y_2} = \frac{z_+ z_- \rho_\mathrm{s} \phi'}{(z_+ - z_-)c - z_+\rho_\mathrm{s}}, \tag{67}$$

$$\frac{\partial f_2}{\partial y_4} = \frac{z_+ z_- \rho_\mathrm{s} c'}{(z_+ - z_-)c - z_+\rho_\mathrm{s}}, \tag{68}$$

$$\frac{\partial f_3}{\partial y_4} = 1, \tag{69}$$

$$\frac{\partial f_4}{\partial y_1} = \frac{(z_+ - z_-)^2 c' \phi'}{[(z_+ - z_-)c - z_+\rho_\mathrm{s}]^2}, \tag{70}$$

$$\frac{\partial f_4}{\partial y_2} = -\frac{(z_+ - z_-)\phi'}{(z_+ - z_-)c - z_+\rho_\mathrm{s}}, \tag{71}$$

$$\frac{\partial f_4}{\partial y_4} = -\frac{(z_+ - z_-)c'}{(z_+ - z_-)c - z_+\rho_\mathrm{s}}, \tag{72}$$

$$\frac{\partial f_5}{\partial y_1} = 1. \tag{73}$$

For galvanostatic conditions, the $\frac{\partial f}{\partial p}$ Jacobian $\in \mathbb{R}^{5\times 1}$ is a zero vector. The nonzero elements of the $\frac{\partial y_\mathrm{BC}}{\partial y(x=0)}$ Jacobian ($\in \mathbb{R}^{6\times 5}$ for galvanostatic conditions or $\in \mathbb{R}^{5\times 5}$ for potentiostatic conditions) are given by:

$$\frac{\partial y_{\mathrm{BC},1}}{\partial y_{0,5}} = 1, \tag{74}$$

$$\begin{aligned}\frac{\partial y_{\mathrm{BC},2}}{\partial y_{0,1}} &= -\beta_\mathrm{D}(z_+ D_{+0} - z_- D_{-0})\phi'(x=0) \\ &\quad + J_0^\mathrm{ref}\left(\frac{\xi_+}{\hat{c}_+^\mathrm{ref}}\right)^{1-\frac{\alpha_1}{2}} (c-\rho_\mathrm{s})^{-\frac{\alpha_1}{2}} \exp(-\alpha_1\eta)\Bigg|_{x=0},\end{aligned} \tag{75}$$

$$\frac{\partial y_{\mathrm{BC},2}}{\partial y_{0,2}} = \beta_\mathrm{D}(D_{-0} - D_{+0}), \tag{76}$$

$$\frac{\partial y_{\mathrm{BC},2}}{\partial y_{0,3}} = J_0^\mathrm{ref}\left[\frac{\xi_+(c-\rho_\mathrm{s})}{\hat{c}_+^\mathrm{ref}}\right]^{1-\frac{\alpha_1}{2}} \{\alpha_1\exp(-\alpha_1\eta) + (2-\alpha_1)\exp[(2-\alpha_1)\eta]\}\Bigg|_{x=0}, \tag{77}$$

$$\frac{\partial y_{\mathrm{BC},2}}{\partial y_{0,4}} = \beta_\mathrm{D}[-(z_+ D_{+0} - z_- D_{-0})c(x=0) + z_+ D_{+0}\rho_\mathrm{s}]. \tag{78}$$

For galvanostatic conditions, the nonzero elements of the $\frac{\partial y_{\text{BC}}}{\partial y(x=1)}$ Jacobian $\in \mathbb{R}^{6\times 5}$ are given by

$$\frac{\partial y_{\text{BC},3}}{\partial y_{1,1}} = z_- \phi'(x=1), \tag{79}$$

$$\frac{\partial y_{\text{BC},3}}{\partial y_{1,2}} = 1, \tag{80}$$

$$\frac{\partial y_{\text{BC},3}}{\partial y_{1,4}} = z_- c(x=1), \tag{81}$$

$$\begin{aligned}\frac{\partial y_{\text{BC},4}}{\partial y_{1,1}} &= \beta_{\text{D}}(z_+ D_{+0} - z_- D_{-0})\phi'(x=1) \\ &\quad + J_0^{\text{ref}} \left(\frac{\xi_+}{\hat{c}_+^{\text{ref}}}\right)^{1-\frac{\alpha_1}{2}} (c-\rho_{\text{s}})^{-\frac{\alpha_1}{2}} \exp(-\alpha_1 \eta)\Bigg|_{x=1},\end{aligned} \tag{82}$$

$$\frac{\partial y_{\text{BC},4}}{\partial y_{1,2}} = -\beta_{\text{D}}(D_{-0} - D_{+0}), \tag{83}$$

$$\frac{\partial y_{\text{BC},4}}{\partial y_{1,3}} = J_0^{\text{ref}} \left[\frac{\xi_+(c-\rho_{\text{s}})}{\hat{c}_+^{\text{ref}}}\right]^{1-\frac{\alpha_1}{2}} \{\alpha_1 \exp(-\alpha_1 \eta) + (2-\alpha_1)\exp[(2-\alpha_1)\eta]\}\Bigg|_{x=1}, \tag{84}$$

$$\frac{\partial y_{\text{BC},4}}{\partial y_{1,4}} = -\beta_{\text{D}}[-(z_+ D_{+0} - z_- D_{-0})c(x=1) + z_+ D_{+0}\rho_{\text{s}}], \tag{85}$$

$$\frac{\partial y_{\text{BC},5}}{\partial y_{1,5}} = 1, \tag{86}$$

$$\frac{\partial y_{\text{BC},6}}{\partial y_{1,1}} = \beta_{\text{D}}(z_+ D_{+0} - z_- D_{-0})\phi'(x=1), \tag{87}$$

$$\frac{\partial y_{\text{BC},6}}{\partial y_{1,2}} = -\beta_{\text{D}}(D_{-0} - D_{+0}), \tag{88}$$

$$\frac{\partial y_{\text{BC},6}}{\partial y_{1,4}} = -\beta_{\text{D}}[-(z_+ D_{+0} - z_- D_{-0})c(x=1) + z_+ D_{+0}\rho_{\text{s}}], \tag{89}$$

and the nonzero element of the $\frac{\partial y_{\text{BC}}}{\partial p}$ Jacobian $\in \mathbb{R}^{6\times 1}$ is given by

$$\frac{\partial y_{\text{BC},4}}{\partial p} = J_0^{\text{ref}} \left[\frac{\xi_+(c-\rho_{\text{s}})}{\hat{c}_+^{\text{ref}}}\right]^{1-\frac{\alpha_1}{2}} \{\alpha_1 \exp(-\alpha_1 \eta) + (2-\alpha_1)\exp[(2-\alpha_1)\eta]\}\Bigg|_{x=1}, \tag{90}$$

while for potentiostatic conditions, the nonzero elements of the $\frac{\partial y_{\mathrm{BC}}}{\partial y(x=1)}$ Jacobian $\in \mathbb{R}^{5\times 5}$ are given by

$$\frac{\partial y_{\mathrm{BC},3}}{\partial y_{1,1}} = z_{-}\phi'(x=1), \tag{91}$$

$$\frac{\partial y_{\mathrm{BC},3}}{\partial y_{1,2}} = 1, \tag{92}$$

$$\frac{\partial y_{\mathrm{BC},3}}{\partial y_{1,4}} = z_{-}c(x=1), \tag{93}$$

$$\begin{aligned}\frac{\partial y_{\mathrm{BC},4}}{\partial y_{1,1}} &= \beta_{\mathrm{D}}(z_{+}D_{+0} - z_{-}D_{-0})\phi'(x=1) \\ &\quad + J_0^{\mathrm{ref}}\left(\frac{\xi_{+}}{\hat{c}_{+}^{\mathrm{ref}}}\right)^{1-\frac{\alpha_1}{2}}(c-\rho_{\mathrm{s}})^{-\frac{\alpha_1}{2}}\exp(-\alpha_1\eta)\bigg|_{x=1},\end{aligned} \tag{94}$$

$$\frac{\partial y_{\mathrm{BC},4}}{\partial y_{1,2}} = -\beta_{\mathrm{D}}(D_{-0} - D_{+0}), \tag{95}$$

$$\frac{\partial y_{\mathrm{BC},4}}{\partial y_{1,3}} = J_0^{\mathrm{ref}}\left[\frac{\xi_{+}(c-\rho_{\mathrm{s}})}{\hat{c}_{+}^{\mathrm{ref}}}\right]^{1-\frac{\alpha_1}{2}}\{\alpha_1\exp(-\alpha_1\eta) + (2-\alpha_1)\exp[(2-\alpha_1)\eta]\}\bigg|_{x=1}, \tag{96}$$

$$\frac{\partial y_{\mathrm{BC},4}}{\partial y_{1,4}} = -\beta_{\mathrm{D}}[-(z_{+}D_{+0} - z_{-}D_{-0})c(x=1) + z_{+}D_{+0}\rho_{\mathrm{s}}], \tag{97}$$

$$\frac{\partial y_{\mathrm{BC},5}}{\partial y_{1,5}} = 1. \tag{98}$$

## III. INITIAL GUESSES AND LOWER AND UPPER BOUNDS FOR FITTING PARAMETERS

Table I lists the initial guesses and lower and upper bounds for the fitting parameters $\tilde{\rho}_{\mathrm{s}}$, $\tau$ (only for CN and PE membranes; fixed at 1 for AAO membranes), $\tilde{J}_0^{\mathrm{ref}}$, $\alpha_1$ and $\epsilon_{\mathrm{p}}$.

Table I. Initial guesses and lower and upper bounds for fitting parameters. Initial guess is the first value, and lower and upper bounds are provided as an interval. Lower and upper bounds for $\epsilon_\mathrm{p}$ for datasets $\mathrm{AAO_1}(+/-)$, $\mathrm{AAO_2}(+/-)$, $\mathrm{CN_1}(+/-)$ and $\mathrm{CN_2}(+/-)$ are based on product specifications.

| Dataset | $\tilde{\rho}_\mathrm{s}$ | $\tau$ | $\tilde{J}_0^\mathrm{ref}$ | $\alpha_1$ | $\epsilon_\mathrm{p}$ |
|---|---|---|---|---|---|
| $\mathrm{AAO_1}(-)$ | $-0.5, (-\infty, 0]$ | 1 (fixed) | $0.5, [0, \infty)$ | $0.5, [0, 1]$ | $0.375, [0.25, 0.5]$ |
| $\mathrm{AAO_1}(+)$ | $1.55, [0, \infty)$ | 1 (fixed) | $0.3, [0, \infty)$ | $0.75, [0, 1]$ | $0.375, [0.25, 0.5]$ |
| $\mathrm{AAO_2}(-)$ | $-0.05, (-\infty, 0]$ | 1 (fixed) | $0.05, [0, \infty)$ | $0.5, [0, 1]$ | $0.375, [0.25, 0.5]$ |
| $\mathrm{AAO_2}(+)$ | $0.25, [0, \infty)$ | 1 (fixed) | $0.05, [0, \infty)$ | $0.65, [0, 1]$ | $0.4, [0.25, 0.5]$ |
| $\mathrm{CN_1}(-)$ | $-0.1, (-\infty, 0]$ | $2, [1, \infty)$ | $6, [0, \infty)$ | $0.5, [0, 1]$ | $0.77, [0.66, 0.88]$ |
| $\mathrm{CN_1}(+)$ | $0.75, [0, \infty)$ | $1.25, [1, \infty)$ | $6, [0, \infty)$ | $1, [0, 1]$ | $0.77, [0.66, 0.88]$ |
| $\mathrm{CN_2}(-)$ | $-0.0125, (-\infty, -0.00625]$ | $1, [1, \infty)$ | $0.7, [0, \infty)$ | $0.75, [0, 1]$ | $0.77, [0.66, 0.88]$ |
| $\mathrm{CN_2}(+)$ | $0.1, [0, \infty)$ | $2, [1, \infty)$ | $0.4, [0, \infty)$ | $0.65, [0, 1]$ | $0.77, [0.66, 0.88]$ |
| PE(−) | $-0.25, (-\infty, 0]$ | $5, [1, \infty)$ | $0.5, [0, \infty)$ | $0.75, [0, 1]$ | $0.47, [0, 1]$ |
| PE(+) | $0.5, [0, \infty)$ | $7, [1, \infty)$ | $0.25, [0, \infty)$ | $0.75, [0, 1]$ | $0.47, [0, 1]$ |
